# Supplementary material for: EDA Corpus: A Large Language Model Dataset for Enhanced Interaction with OpenROAD
Source: arXiv:2405.06676 source file (2024-05-04)
Supplement: Supplementary file 1 [file db.tex]

\begin{lstlisting}[language=Python, caption={Example using native ChatGPT3.5 for querying OpenDB APIs.}]
Prompt: 

You are a coding assistant with specialty in OpenROAD Python API, get the all the unplaced instance as a list.

Response:

import opendbpy as odb

def get_unplaced_instances(db):
    unplaced_instances = []
    
    # Iterate through all instances in the design
    block = db.getChip().getBlock()
    for inst in block.getInsts():
        placement_status = inst.isPlaced()
        if not placement_status:
            unplaced_instances.append(inst)
    
    return unplaced_instances

# Replace 'your_design.db' with the name of your OpenDB database file
db = odb.dbDatabase.open('your_design.db')

unplaced_instances = get_unplaced_instances(db)

# Print unplaced instances
for inst in unplaced_instances:
    print(inst.getName())


\end{lstlisting}
\vspace{-3mm}

\begin{lstlisting}[language=Python, caption={Example using native ChatGPT4 for querying OpenDB APIs.}]
Prompt: 

You are a coding assistant with specialty in OpenROAD Python API, get the all the unplaced instance as a list.

Response:

from openroad import OpenRoad, Design

# Initialize OpenROAD
or_tool = OpenRoad()

# Load your design
design = or_tool.loadDesign("your_design_file.def")

# Access the design database
db = design.getDb()

# Get all instances
instances = db.getChip().getBlock().getInsts()

# Filter unplaced instances
unplaced_instances = [inst for inst in instances if inst.getPlacementStatus() != "PLACED"]

# Convert to a list of instance names (or however you wish to represent them)
unplaced_instance_names = [inst.getName() for inst in unplaced_instances]

# Now unplaced_instance_names contains the names of all unplaced instances

# Example usage
if __name__ == "__main__":
  # Access the OpenROAD design
  design = ord.openroad.design

  # Get the list of all output pins of instances
  output_pins = get_output_pins_of_instances(design)

  # Print the output pins
  print("Output Pins of Instances:")
  for pin in output_pins:
    print(pin)
        
\end{lstlisting}
\vspace{-3mm}

\begin{lstlisting}[language=Python, caption={Example using finetuned ChatGPT3.5 for querying OpenDB APIs.}]
Prompt: 

get the all the unplaced instance as a list.

Response:

# Get the design block
block = ord.get_db_block()
# Get all instances in the block
insts = block.getInsts()
unplaced_instances = []
# Iterate over instances
for inst in insts:
        # Check if the instance is unplaced
        if not inst.isPlaced():
                # Append the instance to the list
                unplaced_instances.append(inst)
return unplaced_instances

\end{lstlisting}
\vspace{-3mm}
