# Supplementary material for: EDA Corpus: A Large Language Model Dataset for Enhanced Interaction with OpenROAD
Source: arXiv:2405.06676 source file (2024-05-04)
Supplement: Supplementary file 2 [file description.tex]

\begin{lstlisting}[language=Python, caption={Example using native ChatGPT3.5 for querying OpenROAD information.}]
Prompt: 

You are an assistant with specialty in knowledge about OpenROAD, what does the report_cell_usage command do?

Response:

In OpenROAD, the report_cell_usage command is used to generate a report that provides information about the usage of cells within a design. This command helps designers analyze how cells are utilized throughout their design, which can be crucial for optimizing performance, reducing area, or improving other aspects of the design.

When you run the report_cell_usage command, it typically generates a report that includes details such as:

Cell Name: The name of each cell used in the design.
Instance Count: The number of instances of each cell used in the design.
Cell Area: The area occupied by each cell, usually in terms of square micrometers or a similar metric.
Percentage of Total Area: The proportion of the total design area occupied by each cell.
Fanout: The number of nets driven by each instance of the cell, providing insights into the connectivity of the design.
Usage Statistics: Additional statistics or metrics related to the usage of each cell, which can vary depending on the specific implementation of the command.
By reviewing the information provided in the report generated by report_cell_usage, designers can identify cells that are heavily utilized or underutilized, allowing them to make informed decisions about design optimization, resource allocation, and other aspects of the design process. This command is particularly valuable in the context of physical design and optimization workflows within the OpenROAD environment.

\end{lstlisting}
\vspace{-3mm}

\begin{lstlisting}[language=Python, caption={Example using native ChatGPT4 for querying OpenROAD information.}]
Prompt: 

You are an assistant with specialty in knowledge about OpenROAD, what does the report_cell_usage command do?

Response:

The report_cell_usage command in OpenROAD, which is a part of the OpenROAD project's suite of tools for automated chip design, is typically used to generate a report detailing the usage of standard cells in the design. This command can be particularly useful for understanding how different types of standard cells (like logic gates, flip-flops, etc.) are distributed across the design, helping designers to evaluate the composition and complexity of their circuit.

The output of the report_cell_usage command usually includes information such as the number of instances of each cell type, the total cell area, and possibly other metrics related to the physical and logical properties of the cells used in the design. This information can aid in optimizing the design for area, power, and performance by identifying opportunities to replace, merge, or remove certain cells.

If you need more detailed, specific information about how to use the report_cell_usage command or its options within the OpenROAD flow, it might be necessary to consult the official OpenROAD documentation or source code, as the capabilities and features of OpenROAD tools can evolve.
        
\end{lstlisting}
\vspace{-3mm}

\begin{lstlisting}[language=Python, caption={Example using finetuned ChatGPT3.5 for querying OpenROAD information.}]
Prompt: 

what does the report_cell_usage command do?

Response:

report_cell_usage command is to report cell usage of the design. It essentially translates the abstract cell into the specific cell that is used.

\end{lstlisting}
\vspace{-3mm}
