# Supplementary material for: EDA Corpus: A Large Language Model Dataset for Enhanced Interaction with OpenROAD
Source: arXiv:2405.06676 source file (2024-05-04)
Supplement: Supplementary file 3 [file flow.tex]

\begin{lstlisting}[language=Python, caption={Example using native ChatGPT3.5 for querying EDA flow APIs.}]
Prompt: 

You are a coding assistant with specialty in OpenROAD Python API, how can I perform IR drop analysis on the M1 layer where the pins are located?

Response:

import openroad as or

# Initialize OpenROAD environment
or_init = or.ord.OpenRoad()
design = "your_design_name"

# Read design
or_init.read_design(design)

# Construct power grid
power_grid = or_init.init_power_grid()

# Estimate or calculate currents (for example, from simulation results)
currents = {net: estimate_current(net) for net in power_grid.get_power_nets()}

# Calculate IR drop
ir_drop_results = {}
for net, current in currents.items():
    voltage_drop = power_grid.calculate_ir_drop(net, current, metal_layer="M1")
    ir_drop_results[net] = voltage_drop

# Visualize and analyze IR drop results
# (visualization code depends on your preference, could use matplotlib or other plotting libraries)
# (analysis could involve identifying hotspots, excessive voltage drops, etc.)

# Print results
for net, voltage_drop in ir_drop_results.items():
    print(f"Net: {net}, IR Drop on M1: {voltage_drop} V")

# Close OpenROAD environment
or_init.finish()



\end{lstlisting}
\vspace{-3mm}

\begin{lstlisting}[language=Python, caption={Example using native ChatGPT4 for querying EDA flow APIs.}]
Prompt: 

You are a coding assistant with specialty in OpenROAD Python API, how can I perform IR drop analysis on the M1 layer where the pins are located?

Response:

from openroad import Openroad

# Initialize OpenROAD
or_app = Openroad()

# Load your design files
or_app.read_lef("path/to/your_file.lef")
or_app.read_def("path/to/your_file.def")
# Example pseudo-code for IR drop analysis setup
# Replace `run_ir_drop_analysis` with the actual OpenROAD command if different.
# Specify the layer and other parameters as needed.
or_app.run_ir_drop_analysis(layer='M1', parameters={...})
# Example pseudo-code to fetch results
results = or_app.get_ir_drop_results()
print(results)
        
\end{lstlisting}
\vspace{-3mm}

\begin{lstlisting}[language=Python, caption={Example using finetuned ChatGPT3.5 for querying EDA flow APIs.}]
Prompt: 

how can I perform IR drop analysis on the M1 layer where the pins are located?

Response:

from openroad import Tech, Design
from pathlib import path
import openroad as ord

tech = Tech()
# Make sure you have files read into OpenROAD DB
design = Design(tech)

# Static IR drop Analysis

psm_obj = design.getPDNSim()
psm_obj.setNet(ord.Tech().getDB().getChip().getBlock().findNet("VDD"))
design.evalTclString(f"psm::set_corner [sta::cmd_corner]")
psm_obj.analyzePowerGrid('', False, '', '')
drops = psm_obj.getIRDropForLayer(tech.getDB().getTech().findLayer("M1"))

\end{lstlisting}
\vspace{-3mm}
