# Supplementary material for: EDA Corpus: A Large Language Model Dataset for Enhanced Interaction with OpenROAD
Source: arXiv:2405.06676 source file (2024-05-04)
Supplement: Supplementary file 4 [file rotate.tex]

\begin{lstlisting}[language=Python, caption={Example using native ChatGPT3.5 for querying Rotation and
Location APIs.}]
Prompt: 

You are a coding assistant with specialty in OpenROAD Python API, horizontally flip the rotation of the instances whose library cell types are 'OR2_X3'.

Response:

import opendbpy as odb

# Open the design
odb_design = odb.dbDatabase.open("your_design.db")

# Get the chip (top level block)
chip = odb_design.getChip()

# Iterate through all instances in the design
for inst in chip.getBlock().getInsts():
    # Check if the library cell type matches 'OR2_X3'
    if inst.getMaster().getCellName() == 'OR2_X3':
        # Flip the rotation horizontally
        bbox = inst.getBBox()
        inst.setOrigin(odb.Point(bbox.xMax(), bbox.yMin()))
        inst.setRotation(odb.dbOrientType.MY)

# Save the modified design
odb_design.save("flipped_design.db")

\end{lstlisting}
\vspace{-3mm}

\begin{lstlisting}[language=Python, caption={Example using native ChatGPT4 for querying Rotation and
Location APIs.}]
Prompt: 

You are a coding assistant with specialty in OpenROAD Python API, horizontally flip the rotation of the instances whose library cell types are 'OR2_X3'.

Response:

import openroad as ord

def flip_horizontal_if_or2_x3(design):
    # Iterate over all instances in the design
    for inst in design.getInstances():
        # Check if the library cell type of the instance is 'OR2_X3'
        if inst.getMaster().getName() == 'OR2_X3':
            # Get the current orientation of the instance
            orientation = inst.getOrientation()
            
            # Dictionary to map current orientation to its horizontal flip
            orientation_flip_map = {
                'R0': 'MY', 'MY': 'R0',
                'R180': 'MX', 'MX': 'R180',
                'R90': 'MYR90', 'MYR90': 'R90',
                'R270': 'MXR90', 'MXR90': 'R270'
            }
            
            # Flip the orientation
            new_orientation = orientation_flip_map.get(orientation, orientation)
            inst.setOrientation(new_orientation)
            print(f"Flipped {inst.getName()} to {new_orientation}")

# Assuming 'design' is your current design object
flip_horizontal_if_or2_x3(design)

\end{lstlisting}
\vspace{-3mm}

\begin{lstlisting}[language=Python, caption={Example using finetuned ChatGPT3.5 for querying Rotation and
Location APIs.}]
Prompt: 

horizontally flip the rotation of the instances whose library cell types are 'OR2_X3'.

Response:

# Horizontally flip the rotation of the instances whose library cell types are 'AND2_X3'

#define flipping function
def flipX(value):
    if value == "R0":
      return "MX"
    elif value == "R90":
      return "MYR90"
    elif value == "R180":
      return "MY"
    elif value == "R270":
      return "MXR90"
    elif value == "MY":
      return "R180"
    elif value == "MYR90":
      return "R90"
    elif value == "MX":
      return "R0"
    elif value == "MXR90":
      return "R270"

# Get the design block
block = design.getBlock()

# Get all instances in the block
insts = block.getInsts()

# Iterate through all instances in the block
for inst in insts:
    # Check if the library cell type is 'AND2_X3'
    if inst.getMaster().getName() == 'OR2_X3':
        # Horizontally flip the rotation of the instance
        orient = inst.getOrient()
        orient = flipX(orient)
        inst.setOrient(orient)

\end{lstlisting}
\vspace{-3mm}
