# Supplementary material for: EDA Corpus: A Large Language Model Dataset for Enhanced Interaction with OpenROAD
Source: arXiv:2405.06676 source file (2024-05-04)
Supplement: Supplementary file 5 [file sizing.tex]

\begin{lstlisting}[language=Python, caption={Example using native ChatGPT3.5 for querying Rotation and
Location APIs.}]
Prompt: 

You are a coding assistant with specialty in OpenROAD Python API, downsize master of instance split30 to BUF_X1.

Response:

import opendbpy as odb

# Load the design
db = odb.dbDatabase.create()
odb.read_lef(db, "your_lef_file.lef")
odb.read_def(db, "your_def_file.def")
design = db.getChip()

# Find the master cell
master_cell = design.findMaster("split30")

if master_cell is not None:
    # Create a new instance of BUF_X1
    buf_x1_master = design.findMaster("BUF_X1")
    if buf_x1_master is not None:
        # Create a new instance of BUF_X1
        buf_x1_instance = odb.dbInst_create(design, buf_x1_master, "BUF_X1_instance")

        # Replace the split30 master cell with BUF_X1 instance
        master_cell.delete()

        # Write changes to the design
        odb.write_def(design, "output.def")

        print("Successfully downsized split30 to BUF_X1.")
    else:
        print("BUF_X1 master not found in the design.")
else:
    print("split30 master cell not found in the design.")


\end{lstlisting}
\vspace{-3mm}

\begin{lstlisting}[language=Python, caption={Example using native ChatGPT4 for querying Rotation and
Location APIs.}]
Prompt: 

You are a coding assistant with specialty in OpenROAD Python API, downsize master of instance split30 to BUF_X1.

Response:

# Assuming 'design' is your current design object
# and 'lib' is the library object containing BUF_X1

# Step 2: Find the instance 'split30'
instance_split30 = design.getInstance("split30")

if instance_split30 is not None:
    # Step 3: Get the 'BUF_X1' master from the library
    buf_x1_master = lib.findMaster("BUF_X1")
    
    if buf_x1_master is not None:
        # Step 4: Downsize the master of 'split30' to 'BUF_X1'
        instance_split30.setMaster(buf_x1_master)
        print("Instance 'split30' has been downsized to 'BUF_X1'.")
    else:
        print("Error: Master 'BUF_X1' not found in the library.")
else:
    print("Error: Instance 'split30' not found in the design.")


\end{lstlisting}
\vspace{-3mm}

\begin{lstlisting}[language=Python, caption={Example using finetuned ChatGPT3.5 for querying Rotation and
Location APIs.}]
Prompt: 

downsize master of instance split30 to BUF_X1.

Response:

# Downsize the master of the instance "split30" to "BUF_X1"

# Get the block of the design
block = design.getBlock()

# Find the instance named "split30"
inst = block.findInst("split30")

# Downsize the master of the instance to "BUF_X1"
inst.downsizeMaster("BUF_X1")

\end{lstlisting}
\vspace{-3mm}
