# Supplementary material for: EDA Corpus: A Large Language Model Dataset for Enhanced Interaction with OpenROAD
Source: arXiv:2405.06676 source file (2024-05-04)
Supplement: Supplementary file 6 [file 7-appendix.tex]

\section{Appendix}
\noindent
Table~\ref{table:appendix_experiment} presents a rudimentary result of searching for OpenROAD Python API sample codes and OpenROAD information using native ChatGPT 3.5/4 and finetuned ChatGPT 3.5s. After finetuning ChatGPT3.5 using $100$ randomly selected prompt-code data points and $150$ question-answer data points, we can achieve $44\%$ accuracy in terms of generating codes can perfectly run. We found that native ChatGPT4 can also generate a few perfectly executable codes, we believe that's because OpenROAD Python APIs are well-named, i.e., the function name resonates with the use case of the function, and with prompting ChatGPT4 using the words existing in the function name, ChatGPT4 can also generate code that can run flawlessly. However, we consider that to be an extreme case.

Although all GPTs can give information about OpenROAD, it's still worth finetuning LLM on our dataset as we can see that the answers become much more straightforward. This response can contain less irrelevant information in real-world use cases and lead to fewer misunderstandings.

\begin{figure}
    \includegraphics[width= 0.99\linewidth]{figs/flow_appendix_1.drawio.png}
    \caption{Example using GPTs for querying EDA flow APIs. Red text means GPT generates API that does not exist.}
    \label{fig:flow_ir_compare}
\end{figure}

\begin{figure}
    \includegraphics[width= 0.99\linewidth]{figs/flow_appendix_2.drawio.png}
    \caption{Example using GPTs for querying EDA flow APIs. Red text means GPT generates API that does not exist.}
    \label{fig:flow_ir_compare}
\end{figure}
