# Supplementary material for: EDA Corpus: A Large Language Model Dataset for Enhanced Interaction with OpenROAD
Source: arXiv:2405.06676 source file (2024-05-04)
Supplement: Supplementary file 7 [file buffer.tex]

\begin{lstlisting}[language=Python, caption={Example using native ChatGPT3.5 for querying EDA flow APIs.}]
Prompt: 

You are a coding assistant with specialty in OpenROAD Python API, add a new instance 'i_am_new_cell' using buffer cell 'i_am_buffer' after the instance 'temp_inst_1' on the net 'temp_net_1', and connect the instances using a new net 'temp_net_2'.

Response:


\end{lstlisting}
\vspace{-3mm}

\begin{lstlisting}[language=Python, caption={Example using native ChatGPT4 for querying EDA flow APIs.}]
Prompt: 

You are a coding assistant with specialty in OpenROAD Python API, add a new instance 'i_am_new_cell' using buffer cell 'i_am_buffer' after the instance 'temp_inst_1' on the net 'temp_net_1', and connect the instances using a new net 'temp_net_2'.

Response:


        
\end{lstlisting}
\vspace{-3mm}

\begin{lstlisting}[language=Python, caption={Example using finetuned ChatGPT3.5 for querying EDA flow APIs.}]
Prompt: 

add a new instance 'i_am_new_cell' using buffer cell 'i_am_buffer' after the instance 'temp_inst_1' on the net 'temp_net_1', and connect the instances using a new net 'temp_net_2'.

Response:


\end{lstlisting}
\vspace{-3mm}
