# Supplementary material for: EDA Corpus: A Large Language Model Dataset for Enhanced Interaction with OpenROAD
Source: arXiv:2405.06676 source file (2024-05-04)
Supplement: Supplementary file 8 [file appendix.tex]

% Please add the following required packages to your document preamble:
% \usepackage{multirow}
%\begin{table}[]
%\caption{Comparison between ChatGPT3.5/4 and finetuned ChatGPT3.5s~\redHL{Bing-Yue this table can be part of the main paper not the appendix. It can be in the impact section.}}
%\label{table:appendix_experiment}
%\begin{tabular}{|c|rr|rr|}
%\hline
%\multicolumn{1}{|l|}{\multirow{2}{*}{}}                                             & \multicolumn{2}{c|}{Prompt-Code}                       & \multicolumn{2}{c|}{Question-Answer}                   \\ \cline{2-5} 
%\multicolumn{1}{|l|}{}                                                              & \multicolumn{1}{c|}{True} & \multicolumn{1}{c|}{False} & \multicolumn{1}{c|}{True} & \multicolumn{1}{c|}{False} \\ \hline
%ChatGPT3.5                                                                          & \multicolumn{1}{r|}{0}    & 50                         & \multicolumn{1}{r|}{10}   & 0                          \\ \hline
%ChatGPT4                                                                            & \multicolumn{1}{r|}{3}    & 47                         & \multicolumn{1}{r|}{10}   & 0                          \\ \hline
%\begin{tabular}[c]{@{}c@{}}ChatGPT3.5 finetuned\\ with prompt-code\end{tabular}     & \multicolumn{1}{r|}{22}   & 28                         & \multicolumn{1}{r|}{NA}   & NA                         \\ \hline
%\begin{tabular}[c]{@{}c@{}}ChatGPT3.5 finetuned\\ with question-answer\end{tabular} & \multicolumn{1}{r|}{NA}   & NA                         & \multicolumn{1}{r|}{10}   & 0                          \\ \hline
%\end{tabular}
%\end{table}
